# Supplementary material for: (Gravitational Wave) Memory of Starobinsky in a Time Crystal (Condensate)
Source: arXiv:2509.21959 source file (2025-09-26)
Supplement: Supplementary file 1 [file Supplgw.tex]

\documentclass{article}
\usepackage{graphicx} % Required for inserting images
\usepackage{subcaption}
\usepackage{float}
\usepackage{geometry}
\geometry{
a4paper, 
textwidth = 506 pt, 
textheight = 714 pt
}
\usepackage{amsmath}
\usepackage{amssymb}
\usepackage{amsfonts}
\usepackage{physics}
\usepackage{xcolor}
\usepackage{appendix}
\usepackage{hyperref}
\hypersetup{
    colorlinks = True,
    linkcolor = blue,
    filecolor = magenta,
    urlcolor = cyan,
    pdftitle = {Overleaf Example}, 
    pdfpagemode = FullScreen
}
\usepackage{comment}
\usepackage{authblk}

\begin{document}

\title{(Gravitational Wave) Memory of Starobinsky in a Time Crystal (Condensate)}

\author[1]{Aurindam Mondal\thanks{\texttt{aurindammondal99@gmail.com}}}
\author[2]{Subir Ghosh\thanks{\texttt{subirghosh20@gmail.com}}} 
\affil{\makebox[\textwidth][c]{\small{$^{1}$Physics and Applied Mathematics Unit, Indian Statistical Institute,}} \newline 
          \makebox[\textwidth][c]{\small{203, Barrackpore Trunk Road, Kolkata, India-         700108.}}}
          
%(Gravitational Wave) Memory of Starobinsky  in a Time Crystal (Condensate  )
%Aurindam Mondal ,  Subir Ghosh
%Indian Statistical Institute,   203, Barrackpore Trunk Road, Kolkata 700108, India

\date{\vspace{-1.4 cm}}

\maketitle

\abstract{In this Letter we have revealed  the presence of Gravitational Wave Memory Effect (GWME) in a new and physically appealing scenario  - the Time Crystal (TC) condensate of Starobinsky Quadratic Gravity. We have used a Gravitational Wave form, induced in a TC condensate in FLRW apacetime, that is much more general than the idealized and somewhat unphysical Plane Wave spacetimes, that are conventionally used. We have presented new results for non-zero  GWME, both  in coordinate and in velocity variables. The results are expressed in Cartesian and Brinkmann coordinates. Approximate analytic forms of transverse geodesics in Brinkmann coordinates are  provided. Very rough quantitative estimates for GWME are also suggested.}

\vspace{0.6 cm}

{\bf{Appendix A: Review of Geometric Condensate and Gravitational wave profile}}\\
Let us give a brief introduction of \textit{Geometric Condensate} constructed from the Starobinsky action in presence of cosmological constant $\Lambda$. First we consider the following quadratic gravity action 
\begin{eqnarray}\label{Starobinsky_action}
    A &=& \frac{1}{16\pi G} \int d^{4}x \sqrt{-g} \left(\mathcal{R} + \alpha \mathcal{R}^{2} - 2\Lambda \right) . 
\end{eqnarray}
Here $\mathcal{R}$ is the Ricci scalar of the given spacetime and $\alpha$ be a small, coupling constant with some appropriate dimension i.e. $[\alpha] = [L^{2}]$. 

Now we want to see the structure of the above action Eq. (\ref{Starobinsky_action}) under first order metric perturbation. Generally the linear order metric perturbation is introduced in the following manner
\begin{eqnarray}
    g_{\mu\nu} &=& \Tilde{g}_{\mu\nu} + h_{\mu\nu} \, , 
\end{eqnarray}
where $\Tilde{g}_{\mu\nu}$ be any spacetime dependent background metric, however we restrict ourselves to dS or AdS case only and $h_{\mu\nu}$ represents small metric perturbation over the smooth background. Furthermore, the metric perturbations $h_{\mu\nu}$ can be decomposed again in terms of the irreducible components of Rotation group as follows, 
\begin{eqnarray}
    h_{\mu\nu} &=& h^{TT}_{\mu\nu} + \big(\widetilde{\nabla}_{\mu}v_{\nu} + \widetilde{\nabla}_{\nu}v_{\mu} \big) + \big(\widetilde{\nabla}_{\mu} \widetilde{\nabla}_{\nu} - \frac{1}{4} g_{\mu\nu} \widetilde{\Box} \big) v + \frac{1}{4} \widetilde{g}_{\mu\nu} h \, . 
\end{eqnarray}
Here $v$ represents the scalar, $v_{\mu}$ represents the vector and $h^{TT}_{\mu\nu}$ denotes the traceless-transverse part of the second rank tensorial degree of freedom. The main advantage of this irreducible decomposition is that it cannot be broken further into some more fundamental degrees of freedom. 

Up to second order metric perturbations, the Starobinsky action Eq. (\ref{Starobinsky_action}) can be completely decoupled into two independent portions. One corresponds to the conventional spin-$2$ tensorial degree of freedom $h^{TT}_{\mu\nu}$, known as \textit{graviton} and other corresponds to a spin-$0$ scalar field configuration $\phi$. The final decoupled form of the Starobinsky action is given below, 
\begin{eqnarray}
    A &=& \frac{1}{16\pi G} \int d^{4}x \sqrt{-\widetilde{g}} \hspace{0.1cm} \bigg[\frac{1}{4} \big(1 + 32\pi G\alpha\widetilde{R}_{0} \big) \hspace{0.06cm} h^{\mu\nu}_{TT} \bigg(\widetilde\Box - \frac{\widetilde{R}_{0}}{6} \bigg) h^{TT}_{\mu\nu} \nonumber \\ 
    && + \hspace{0.1cm} 9\pi G\alpha \bigg(\widetilde{\Box}\phi + \frac{\widetilde{R}_{0}}{3} \phi \bigg)^{2} - \frac{3}{32} \big(1 + 32\pi G\alpha\widetilde{R}_{0} \big) \hspace{0.06cm} \phi \bigg(\widetilde{\Box} + \frac{\widetilde{R}_{0}}{3} \bigg) \phi \bigg] \, . 
\end{eqnarray}
Here $\Tilde{R}_{0}$ denotes the constant curvature of background spacetime and the scalar field configuration $\phi$ is defined as follows: $\phi := (h - \widetilde{\Box}v)$. We coined the term \textit{``Geometric Condensate (GC)"} for the scalar field $\phi$, since it is constructed completely from the geometric degrees of freedom of the metric perturbation $h_{\mu\nu}$.  

Our next task is to map the decoupled action associated with \textit{Geometric Condensate} (GC) into a generic action of higher derivative scalar and then determine the corresponding stress-energy tensor $T_{\mu\nu}$. First, we choose a generic action associated with higher derivative scalar in the following manner [1]
\begin{eqnarray}
    S &=& -\frac{1}{2} \int d^4x~\sqrt{-g} \bigg[(\Box\phi)^2+(m_1^2+m_2^2)g^{\mu\nu} \nabla_{\mu}\phi \nabla_{\nu}\phi + m_1^2m_2^2 \hspace{0.06cm} \phi^2 \bigg] , 
\end{eqnarray}
where $(m_{1}, m_{2})$ are two distinct, real quantities having the mass dimension. After some algebraic manipulations, the action associated with GC becomes the following 
\begin{eqnarray}\label{map_action}
    A_{GC} &=& \frac{9\alpha}{156\pi G} \int d^4x \sqrt{-\widetilde g} \left[(\widetilde{\Box} \phi )^2 -\frac{\widetilde{R}_{0}}{18\alpha}\phi^{2} + \left(\frac{\widetilde{R}_{0}}{3}-\frac{1}{6 \alpha} \right) \phi\widetilde{\Box}\phi \right] . 
\end{eqnarray}
For simplicity, we are going to drop the tilde symbol from the background quantities. From the usual definition, the energy-momentum tensor of the above mentioned generic action Eq. (\ref{map_action}) is found to be the following 
\begin{eqnarray}
    T_{\mu\nu} &=& \frac{9\alpha}{128\pi G} \bigg[ -(\partial_\mu\Box\phi)\partial_\nu\phi \, - \, (\partial_\nu\Box\phi)\partial_\mu\phi \, + \, \frac{g_{\mu\nu} (\Box\phi)^2}{2} \, + \, \frac{\widetilde{R}_{0}}{36\alpha} g_{\mu\nu}\phi^2 \nonumber \\ 
    && \hspace{0.1cm} + \, \hspace{0.1cm} g_{\mu\nu} g^{\alpha\beta}(\partial_\alpha\Box\phi )\partial_\beta\phi \, + \, \left(\frac{1}{6 \alpha} - \frac{\widetilde{R}_{0}}{3} \right) \bigg(\partial_\mu\phi\partial_\nu\phi -\frac{1}{2}g_{\mu\nu}g^{\alpha\beta}\partial_\alpha \phi\partial_\beta\phi \bigg) \bigg] .
\end{eqnarray}
Once $T_{\mu\nu}$ associated with GC has been found, using the minimisation of energy density $T_{00}$ in the Fourier space as described in [2], one finds the following solution for GC
\begin{eqnarray}
    \phi &=& \phi_{0} \cos{\left(\omega\eta \right)} \hspace{0.5cm} ; \hspace{0.5cm} \omega \hspace{0.1cm} = \hspace{0.1cm} a(\eta) \, \sqrt{\frac{R_{0}}{3}} \, . 
\end{eqnarray}
Remember that the authors [2] have used spatially flat FLRW metric as a background geometry during the derivation of the above ansatz for $\phi$. 

Solving the Friedmann equations in presence of  the Time Crystalline (or Geometric) Condensate, acting as matter source,  the scale factor out turns to be, 
\begin{eqnarray}\label{scale_factor}
    a(t) &=& \bigg[\big\{a^{2}(t_{0}) + 8 \big(\alpha R_{0} \big)^{3/4} \big\} \cosh{\bigg\{ 2 \sqrt{\frac{R_{0}c^{2}}{192}} (t-t_{0}) \bigg\}} - 8 \big(\alpha R_{0} \big)^{3/4}  \nonumber \\ 
    && + ~\sqrt{a^{4}(t_{0}) + 16a^{2}(t_{0}) \big(\alpha R_{0} \big)^{3/4} + 2\alpha R_{0}} \hspace{0.1cm} \sinh{\bigg\{2 \sqrt{\frac{R_{0}c^{2}}{192}} (t-t_{0}) \bigg\}} \bigg]^{\boldsymbol{1/2}} \nonumber \\ 
    a(t) &\approx& a(t_{0}) \sqrt{1 + 2 H_{0}(t-t_{0})} . 
\end{eqnarray}
From linearized Einstein field equations, the Gravitational Wave solution (propagating in a FLRW universe) is recovered [3],  
\begin{eqnarray}
    \tilde{h}_{22} \hspace{0.1cm} = \hspace{0.1cm} \tilde{h}_{23} &\approx& c_{3} c_{2} \hspace{0.1cm} e^{-A+A\ln{(A)}} \bigg(\frac{2 \sqrt{41\Omega_{\lambda}}}{A^{1/3}} \bigg)^{3/4} \hspace{0.1cm} \frac{e^{-i\sqrt{\Gamma}x}}{\sqrt{4\Delta t}} \hspace{0.1cm} \sin{\bigg\{\omega(t) \Delta t - (4A+1)\frac{\pi}{4} \bigg\}} \, . 
\end{eqnarray}
Choosing the Synchronous gauge allows us to  reduce the independent degrees of freedom of the metric perturbation from ten to two:
\begin{equation}
    \tilde{h}_{0\mu} \hspace{0.1cm} = \hspace{0.1cm} \tilde{h}_{1\mu} \hspace{0.1cm} = \hspace{0.1cm} 0 \hspace{0.5cm} ; \hspace{0.5cm} \tilde{h}_{22} \hspace{0.1cm} = \hspace{0.1cm} - \tilde{h}_{33} \, .  
\end{equation}
\vspace{.3cm}

{\bf{Appendix B: Diagonalizing the transverse sector}} \\ 

We want to diagonalise the symmetric $2\times 2$ matrix
\begin{equation}
g=\begin{pmatrix} a & c \\[4pt] c & b \end{pmatrix}
\end{equation}
having eigenvalues
\begin{equation}
\lambda_{\pm} = \frac{a+b}{2} \;\pm\; \sqrt{\left(\frac{a-b}{2}\right)^2 + c^2}.
\end{equation}
Introduce a rotation
\begin{equation}
R = \begin{pmatrix} \cos\theta & -\sin\theta \\[4pt] \sin\theta & \cos\theta \end{pmatrix},
\end{equation}
with $\theta$ chosen such that
\begin{equation}
\tan(2\theta) = \frac{2c}{\,a-b\,}.
\end{equation}
Explicit Computation of $R^{T} g R$ yields
\begin{equation}
R^{T} g R =
\begin{pmatrix}
a\cos^2\theta + b\sin^2\theta + c\sin 2\theta &
\dfrac{b-a}{2}\sin 2\theta + c\cos 2\theta \\[10pt]
\dfrac{b-a}{2}\sin 2\theta + c\cos 2\theta &
a\sin^2\theta + b\cos^2\theta - c\sin 2\theta
\end{pmatrix}.
\end{equation}
Choose  $\theta$ such that  the off-diagonal terms vanish,
\begin{equation}
\dfrac{b-a}{2}\sin 2\theta + c\cos 2\theta = 0.
\end{equation}
resulting in 
\begin{equation}
R^{T} g R =
\begin{pmatrix}
\lambda_{+} & 0 \\[6pt]
0 & \lambda_{-}
\end{pmatrix}.
\end{equation}
Eigenvectors For each eigenvalue $\lambda$  are obtained by solving
\begin{equation}
\begin{pmatrix} a-\lambda & c \\[4pt] c & b-\lambda \end{pmatrix}
\begin{pmatrix} x \\[4pt] y \end{pmatrix} = 0.
\end{equation}
Convenient choices are
\begin{align}
v_{\lambda} &= 
\begin{pmatrix} c \\[4pt] \lambda - a \end{pmatrix}
\quad \text{or equivalently} \quad
v_{\lambda} = 
\begin{pmatrix} \lambda - b \\[4pt] c \end{pmatrix}.
\end{align}
giving the unnormalised eigenvectors corresponding to $\lambda_{+}$ and $\lambda_{-}$ 
\begin{align}
v_{+} &= \begin{pmatrix} c \\[4pt] \lambda_{+} - a \end{pmatrix}, \\[8pt]
v_{-} &= \begin{pmatrix} c \\[4pt] \lambda_{-} - a \end{pmatrix}.
\end{align}
Normalising these will provide  an orthonormal basis, which coincides with the columns of the rotation matrix $R$. \\ 

{\bf{Appendix C: Explicit form of the $k_{i}$'s:}} \\ 

The explicit form of the coefficients appear in the approximate form of y-geodesic, are given below
\begin{eqnarray}
    k_1 &=& \frac{\beta ^2 \sqrt{\Gamma } c_{0} p_{y0} \omega  (7.667\,  \alpha -10.843\, \mu ) \Omega_{\lambda} \cos{\theta} \,  \sin \left(\frac{\alpha  \sqrt{\Gamma }}{\sqrt{2}}\right) e^{-\frac{\alpha ^2-2 \sqrt{2}\,  \alpha \, \mu +2\, \mu ^2}{4 \sigma ^2}}}{a_{0}^4 \sigma ^3} \nonumber \\ 
    k_2 &=& \frac{\beta ^2 \sqrt{\Gamma } c_{0} p_{y0} \omega^{2} (3.833\,  \alpha -5.421\, \mu ) \Omega_{\lambda} \sin{\theta} \, \sin \left(\frac{\alpha  \sqrt{\Gamma }}{\sqrt{2}}\right) e^{-\frac{\alpha ^2-2 \sqrt{2}\,  \alpha \, \mu +2\, \mu ^2}{4 \sigma ^2}}}{a^{4}_{0} \sigma^{3}} \nonumber \\ 
    k_3 &=& \hspace{-0.1 cm} \frac{\beta  c_{0} p_{y0} \Omega_{\lambda} \sin{\theta} \,  e^{-\frac{\alpha ^2-2 \sqrt{2}\,  \alpha \, \mu +2\, \mu ^2}{4 \sigma ^2}} \left\{\sqrt{\Gamma } \sin \left(\frac{\alpha  \sqrt{\Gamma }}{\sqrt{2}}\right) \left(-7.667\,  \alpha \, \beta +10.843\, \beta \, \mu -7.667 \, \sigma ^2 \omega ^2\right)+\omega ^2 (7.667\, \mu -5.421\,  \alpha ) \cos \left(\frac{\alpha  \sqrt{\Gamma }}{\sqrt{2}}\right) \right\}}{a_{0}^4 \sigma ^3} \nonumber \\ 
    k_4 &=& \frac{c_{0} p_{y0} \Omega_{\lambda} \sin{\theta} \,  e^{-\frac{\alpha ^2-2 \sqrt{2}\,  \alpha \, \mu +2\, \mu ^2}{4 \sigma ^2}} \left\{\cos \left(\frac{\alpha  \sqrt{\Gamma }}{\sqrt{2}}\right) \left(10.843\,  \alpha \, \beta -15.334\, \beta \, \mu +10.843 \, \sigma ^2 \omega ^2\right)+15.334\, \beta  \sqrt{\Gamma } \sigma ^2 \sin \left(\frac{\alpha  \sqrt{\Gamma }}{\sqrt{2}}\right) \right\}}{a_{0}^4 \sigma ^3} \nonumber \\ 
    k_5 &=& -\frac{21.686 c_{0} p_{y0} \sin{\theta} \cos \left(\frac{\alpha  \sqrt{\Gamma }}{\sqrt{2}}\right) e^{-\frac{\alpha ^2-2 \sqrt{2}\,  \alpha \, \mu +2\, \mu ^2}{4 \sigma ^2}}}{a_{0}^4 \sigma ^3} \nonumber \\  
    k_6 &=& \frac{\beta  c_{0} p_{y0} \omega  \Omega_{\lambda} \cos{\theta} \,  e^{-\frac{\alpha ^2-2 \sqrt{2}\,  \alpha \, \mu +2\, \mu ^2}{4 \sigma ^2}} \left\{(15.334\, \mu -10.843\,  \alpha ) \cos \left(\frac{\alpha  \sqrt{\Gamma }}{\sqrt{2}}\right)-15.334 \sqrt{\Gamma } \sigma ^2 \sin \left(\frac{\alpha  \sqrt{\Gamma }}{\sqrt{2}}\right)\right\}}{a_{0}^4 \sigma ^3} + \frac{1.6007 p_{y0} \sqrt{\Omega _{\lambda }}}{a_{0}^2} \nonumber \\ 
    k_7 &=& \frac{21.686 c_{0} p_{y0} \omega  \Omega_{\lambda} \cos{\theta} \,  \cos \left(\frac{\alpha  \sqrt{\Gamma }}{\sqrt{2}}\right) e^{-\frac{\alpha ^2-2 \sqrt{2}\,  \alpha \, \mu +2\, \mu ^2}{4 \sigma ^2}}}{a_{0}^4 \sigma ^3} \, . 
\end{eqnarray}
The other parameters $(\alpha,\, \beta, c_{0}, d_{0})$ are defined as follows, 
\begin{eqnarray}
   \,  \alpha &=& \frac{2 H_{0} t_{0}-1}{\sqrt{2} H_{0} t_{0}} \hspace{0.6 cm} , \hspace{0.6 cm} \beta \hspace{0.1 cm} = \hspace{0.1 cm} \frac{\sqrt{2}}{H_{0} t_{0} \sqrt{41 \Omega _{\lambda }}} \hspace{0.6 cm} , \hspace{0.6 cm} \omega \hspace{0.1 cm} = \hspace{0.1 cm} 2 \sqrt{A_{1}} \hspace{0.6 cm} , \hspace{0.6 cm} \theta \hspace{0.1 cm} = \hspace{0.1 cm} (4A_{1} + 1) \frac{\pi}{4} \, , \nonumber \\  
    A_{1} &=& \frac{4 \Gamma  t_{0}^2 - 27 \Omega_k (a_{0} H_{0} t_{0})^2}{8 \sqrt{41 \Omega _{\lambda }} (a_{0} H_{0} t_{0})^2} \hspace{0.6 cm} , \hspace{0.6 cm} c_{0} \hspace{0.1 cm} = \hspace{0.1 cm} c_{3} c_{2} \, \exp{-A_{1} (1 - \log{A_{1}})} \left(\frac{2 \sqrt{41 \Omega _{\lambda }}}{\sqrt[3]{A_{1}}}\right)^{3/4} \, , \nonumber \\ 
    d_{0} &=& \frac{15}{\sqrt{2 \pi } \sigma } \exp{-\frac{\left(\frac{\alpha + \beta \, \text{$\delta $u}}{\sqrt{2}}-\mu \right)^2}{2 \sigma ^2}} \, . 
\end{eqnarray}

\vspace{.3 cm}

{\bf{References}:} \\ 
1. G. W. Gibbons, C. N. Pope, and S. Solodukhin, Phys. Rev. D 100, 105008 (2019), arXiv:1907.03791 [hep-th]. \\
2.  S.Chakraborty and S.Ghosh, Phys.Dark Univ.35, 100976(2022), arXiv:2001.04680 [gr-qc]. \\ 
3. A. Mondal, S. Ghosh, Gravitational wave propagation in a geometric condensate in Starobinsky cosmology,  Eur.Phys.J.C 85 (2025) 6, 675, e-Print: 2501.11694 [gr-qc].

\end{document}
